# Supplementary material for: AutoTVG: A New Vision-language Pre-training Paradigm for Temporal Video Grounding
Source: arXiv:2406.07091 source file (2024-06-11)
Supplement: Supplementary file 1 [file appendix.tex]

\section{Appendix}

\subsection{Appendix A}

xxx
